# Supplementary material for: Label Super Resolution with Inter-Instance Loss
Source: arXiv:1904.04429 source file (2020-01-07)
Supplement: Supplementary file 1 [file APPENDICES.tex]

\noindent\textbf{{\large APPENDICES}}

\section{Assumption made during the computation of intra-instance variance}

In the Intra-instance loss, the variance of label counts $c_l$ is computed using the following equation (also Eq. 3 in the main submission):
\begin{equation}
\label{eq:assumed-equation}
\centering
\sigma_{l,z,k}^2= \frac{1}{| X_k |^2} \sum_{i,j} \Big (p(y_{i,j}=l\mid X_k, z) \times \big(1-p(y_{i,j}=l\mid X_k, z)\big)\Big ).
\end{equation}

Eq. \ref{eq:assumed-equation} assumes that $y_{i,j}$ for $i,j \in X_k$ are independent with each other. We explain this in detail:

Let $n \in[1,|X_k|]$ be a condensed index representing $i,j$, and $W_n=\mathbbm{1} (y_{i,j}=l \mid X_k, z)$ where $\mathbbm{1}(\cdot)$ is the indicator function. Then

\begin{equation}
\label{eq:before-assumeption}
\centering
\begin{split}
\sigma_{l,z,k}^2= Var(\frac{1}{\left | X_k \right |} \sum_{n=1}^{\left | X_k \right |} W_n)
=\frac{1}{\left | X_k \right |^2}(\sum_{n=m} Cov(W_n,W_m)+\sum_{n\neq m}Cov(W_n,W_m))\\
=\frac{1}{\left | X_k \right |^2}(\sum_{n=1}^{\left | X_k \right |}Var(W_n)+\sum_{n\neq m}Cov(W_n,W_m)).
\end{split}
\end{equation}

By assuming that $W_n$ are independent from each other, we have $Cov(W_n,W_m)=0$ for all $n \neq m$. Thus,

\begin{equation}
\label{eq:after-assumption}
\centering
\begin{split}
\sigma_{l,z,k}^2
=\frac{1}{\left | X_k \right |^2}(\sum_{n=1}^{\left | X_k \right |}Var(W_n)
= \frac{1}{| X_k |^2} \sum_{i,j} \Big (p(y_{i,j}=l\mid X_k, z) \times \big(1-p(y_{i,j}=l\mid X_k, z)\big)\Big ).
\end{split}
\end{equation}\label{eq:3}

In practice, the assumption that $W_n$ are independent from each other are usually not true. In other words, there exists $Cov(W_n,W_m) > 0$ for some $n \neq m$. As a result, the value of Eq. \ref{eq:after-assumption} is strictly smaller than the true variance in Eq. \ref{eq:before-assumeption}.

The statistics matching process is trying to match the variance computed by Eq. \ref{eq:after-assumption} to the empirical variance. Since Eq. \ref{eq:after-assumption} would be smaller than the empirical variance, directly matching them would introduce bias. Let 
\begin{equation}
\alpha = \sum_{n=1}^{\left | X_k \right |}Var(W_n)/(\sum_{n=1}^{\left | X_k \right |}Var(W_n)+\sum_{n\neq m}Cov(W_n,W_m)), \quad \alpha \in [0,1],
\end{equation}
and denote the empirical variance as $V_e$. We can match the value of equation \ref{eq:before-assumeption} with $\alpha \times V_e$. The optimal value of $\alpha$ depends on the distribution of data.

For the Intra-instance LSR baseline, instead of matching ($\mu_{l,z,k}$, $\sigma_{l,z,k}$) with ($\eta_{l,z,k}$, $\rho_{l,z,k}$) respectively by the equation (5) in the original submission, we match ($\mu_{l,z,k}$, $\sigma_{l,z,k}$) with ($\eta_{l,z,k}$, $\alpha \times \rho_{l,z,k}$) respectively. The hyperparameter $\alpha$ is selected via experiments. Note that this $\alpha$ term is not presented nor used in the original Intra-instance LSR paper \cite{malkin19label}.

In the proposed Intra+inter-instance LSR setting, the variance is computed by Eq. (11) in the original submission as follows:
\begin{equation}
\begin{split}
\sigma_{l,z}^{2}
= & \frac{1}{N}\sum_{k=1}^{N}\sigma_{l,z,k}^2+ \frac{1}{N}\sum_{k=1}^{N}(\mu_{l,z,k}^2 -\mu_{l,z}^2) \text{.}
\end{split}
\end{equation}
Here $\sigma_{l,z,k}$ is also computed by Eq. \ref{eq:after-assumption}. Thus, it is also strictly smaller than the actual $\sigma_{l,z,k}$ in real world datasets. Then $\sigma_{l,z}$ is also smaller than the actual $\sigma_{l,z}$. In our experiments, we also select the hyperparameter $\alpha$ for matching ($\mu_{l,z,k}$, $\sigma_{l,z,k}$) with ($\eta_{l,z,k}$, $\alpha \times \rho_{l,z,k}$) respectively. To investigate the influence of $\alpha$  on the final performance of different models. We test different values of $\alpha$ on the breast cancer segmentation task and the results are shown in Tab. \ref{tab:ab}. 
We see that for the breast cancer segmentation task, the best $\alpha$ is $0.8$.

\begin{table}[]
\centering
\begin{tabular}{rlllll}
$\alpha=$     & 0.2 & 0.4   & 0.6 & 0.8 & 1.0  \\\hline\hline
%Intra-instance loss (Masked IoU)      &  0.5998  & 0.6208    &   \textbf{0.6317}   &  0.5751  &  -   \\\hline
%Intra+inter instance loss (Masked IoU) &   - & 0.5753   & 0.5725    &\textbf{ 0.6275}    &    0.6158  \\\hline

Intra+inter instance loss (Masked IoU) &   0.5656& 0.5753   &   0.5716  &\textbf{ 0.6275}    &     0.6223 \\\hline
\end{tabular}\caption{The performance of the proposed Inter+intra-instance LSR for the breast cancer segmentation task with different scale factors $\alpha$ for scaling the ground truth empirical standard deviation.}
\end{table}\label{tab:ab}

%The empirical mean and variance used in this experiments for training  are from visual approximation, the visual approximation is detailed in Sec. \ref{sec:visual}.

\section{Results using alternative ground truth label counts}\label{sec:visual}

The label super resolution network is trained using the conditional distribution $p(c_l \mid  z)$ which is the distribution of label counts $c_l$ within an image block with given low resolution label $z$. 

\subsection{Visually approximating ground truth label counts}
In the main submission we show a less accurate but faster way of obtaining $p(c_l|z)$. We call this process \textbf{visual approximation}. The process of it is as follows: A domain expert visually approximates the count of pixels $c_l$ without drawing the exact cancer mask. The count of the rest pixels in the image would be the count of pixels for the non-cancer region. The distributions of $c_l$ for each low resolution class is the visually approximated $p(c_l|z)$, as shown in Table \ref{tab:cancer_mu_sigma_estimated}.

\subsection{Estimating ground truth label counts using masks}
In practice, training with visually approximated $p(c_l|z)$ would save annotation time but may impede the performance of the model. Thus, we also show performance of the models trained with mask estimated $p(c_l|z)$. We call this process \textbf{mask estimation}. The process is as follows: A domain expert draws an accurate mask of cancer regions for each image block. Then the count of pixels $c_l$ for a class $l$ (such as cancer or non-cancer) is directly computed from the mask of this image block. Given a low resolution label $z$, the mask estimated distribution of $c_l$ can be computed, as shown in Table \ref{tab:cancer_mu_sigma_accurate}.

For both visual approximation and mask estimation methods, we extracted 12-20 blocks for each of the $10$ low resolution classes. A total number of $167$ blocks are extracted. For each low resolution label $z$, we extract at most one image block with label $z$, per WSI. %For a low resolution class $z$, each block is extracted from a whole-slide image that is different from the source of any other block. 

\subsection{Results of visual approximation and mask estimation}

The time consumed to visually approximate the count for all the $167$ images and draw the cancer masks for all the images is shown in Table \ref{tab:time_consumption}. From the table we can see that the mask drawing time for an image is $2.4$ times the visual approximation time. It should  be noted that training a deep model using pixel-level supervision that can generalize well to different slides requires many more drawn masks. The time of drawing 167 blocks here is still much less than the actual annotation time for training a traditional pixel-level supervised semantic segmentation model. We also show the performance of the model trained only with those 167 blocks with high resolution supervision in the second row of Table \ref{tab:qualtitative}.

The performance of models trained using the visually approximated $p(c_l|z)$, the mask estimated $p(c_l|z)$ and limited high resolution supervision are in  Table \ref{tab:qualtitative}. We can see that for Intra-instance LSR, mask estimation does not significantly improve the performance. For intra+inter-instance LSR, mask estimation significantly improves the performance. As a result, with mask estimated $p(c_l|z)$, the intra+inter-instance LSR outperforms the intra-instance LSR significantly. Both of the LSR methods outperform the low resolution labels (the first row in the table) which shows the effectiveness of label super resolution. And both of the LSR methods outperform the model trained with the  167 blocks with pixel-level supervision, this shows that training a pixel-level supervised semantic segmentation model requires large amount of pixel-level super vision. Limited amount of pixel-level super vision may lead to overfitting.
%With the same limited number of blocks for visual approximating the  $p(c_l|z)$, LSR methods also outperform the pixel-level supervised  semantic segmentation method.

%\section{Inter-rater agreement for cancer area estimation}

%Since the count $c_l$ for class $l$ given $z$ is estimated by experts, the estimation between experts may vary. To investigate how the performance of the breast cancer segmentation model would change with different $p(c_l|z)$ estimated by different experts. Two experts look through 196 patches, about 20 patches for each class $z$, to estimate $p(c_l|z)$. The estimated results are shown in Table \ref{tab:cancer_mu_sigma_mao} and Table \ref{tab:cancer_mu_sigma_le}. 

%The total time takes for the estimating process for the two experts are recorded. The first expert takes $17.8$s on average for a patch and the second expert takes $12.55$ s on average for a patch.One of these time segments would be the extra annotation time for super resolving patch level annotations to higher resolution labels. Comparing to  It's an order less than the time would take for pixel-level annotation used in the traditional semantic segmentation methods.

%The the breast cancer segmentation model is trained using the two tables as ground truth, the performance on the test set are in Table \ref{}.

\begin{table}[ht]
\centering
\begin{tabular}{ c | c c }
Image block with & \multicolumn{2}{c}{Count\% of } \\
low resolution class $z$: & \multicolumn{2}{c}{high resolution class $l$:} \\ \cline{2-3}
probability\% as cancer block & Cancer & Non-cancer \\ \hline\hline
0-20  & $4.25 \pm 8.64$ & $95.75 \pm  8.64$ \\ \hline
 20-30 & $2.45\pm 6.43$ & $97.55\pm 6.43$ \\ \hline
 30-40 & $7.92 \pm 7.39$ & $92.08 \pm 7.39$ \\ \hline
 40-50 & $7.00 \pm 10.75$ & $93.00 \pm 10.75$ \\ \hline
 50-60 & $13.00 \pm 14.74$ & $87.00 \pm 14.74$ \\ \hline
60-70   & $6.69 \pm 8.17$ & $93.31 \pm 8.17$ \\ \hline
70-80 & $9.81 \pm13.19$ & $90.19 \pm 13.19$ \\ \hline
 80-90  & $16.56 \pm  21.96$ & $83.44 \pm 21.96$ \\ \hline
 90-95 & $17.72 \pm 27.42$ & $82.28 \pm 27.42$ \\ \hline
 95-100& $49.94 \pm 29.13$ & $50.06 \pm 29.13$ \\ \hline
\end{tabular}
\vspace{0.2cm}
\caption{\label{tab:cancer_mu_sigma_estimated} The mean\% $\pm$ standard deviation\% of the visually approximated count (in percentage) of high resolution labels $l$ in image blocks with low resolution labels $z$.}
\end{table}

\begin{table}[ht]
\centering
\begin{tabular}{ c | c c }
Image block with & \multicolumn{2}{c}{Count\% of } \\
low resolution class $z$: & \multicolumn{2}{c}{high resolution class $l$:} \\ \cline{2-3}
probability\% as cancer block & Cancer & Non-cancer \\ \hline\hline
0-20  & $3.39 \pm 7.95$ & $96.61 \pm  7.95$ \\ \hline
 20-30 & $8.50\pm 8.67$ & $91.50\pm 8.67$ \\ \hline
 30-40 & $11.06 \pm 11.23$ & $88.94 \pm 11.23$ \\ \hline
 40-50 & $8.78 \pm 11.49$ & $91.22 \pm 11.49$ \\ \hline
 50-60 & $10.67 \pm 16.08$ & $89.33 \pm 16.08$ \\ \hline
60-70   & $4.67 \pm 5.15$ & $95.33 \pm 5.15$ \\ \hline
70-80 & $11.27\pm 11.01$ & $88.73 \pm 11.01$ \\ \hline
 80-90  & $18.55 \pm 23.12$ & $81.45 \pm 23.12$ \\ \hline
 90-95 & $25.01 \pm 33.76$ & $74.99 \pm 33.76$ \\ \hline
 95-100& $52.53 \pm 30.69$ & $47.47 \pm 30.69$ \\ \hline
\end{tabular}
\vspace{0.2cm}
\caption{\label{tab:cancer_mu_sigma_accurate} The mean\% $\pm$ standard deviation\% of the mask estimated count (in percentage) of high resolution labels $l$ in image blocks with low resolution labels $z$.}
\end{table}

\begin{table}[]\centering 
\begin{tabular}{l c c}
            &  Visual approximation & Drawing masks\\ \hline \hline
Time for 167 images  &  56 min 32s & 136 min 17s\\ \hline
Average time for 1 image   & 20.3s & 48.96s\\ \hline

\end{tabular}
\vspace{0.2cm}
\caption{\label{tab:time_consumption} The time consumption for two different methods of estimating $p(c_l|z)$.
}
\end{table}

\begin{table}[]\centering 
\begin{tabular}{l c c}
            &  Masked  IoU & Masked DICE\\ \hline \hline
Low resolution model  &  0.5722 &0.7279\\ \hline
Model trained with limited high-res supervision  & 0.5507 & 0.7103\\ \hline
Intra-instance LSR (visually approximated $p(c_l|z)$)   & 0.5827 & 0.7363\\ \hline
Intra-instance LSR (mask estimated $p(c_l|z)$)   &0.5832 & 0.7367\\ \hline
%Inter-instance    & 0.4981 &  0.6650\\ \hline
Intra+inter-instance LSR  (visually approximated $p(c_l|z)$)  &0.5850&0.7381\\ \hline
Intra+inter-instance LSR  (mask estimated $p(c_l|z)$) & 0.6315& 0.7741 \\ \hline
\end{tabular}
\vspace{0.2cm}
\caption{\label{tab:qualtitative} Quantitative results for cancer segmentation in pathology slides. The masked IoU/DICE is computed only in areas around cancer/non-cancer boundaries. It evaluates label super resolution methods in areas that are within a distance of 240 pixels (1000 microns, width of an input patch) away from the ground truth cancer/non-cancer boundaries.
}
\end{table}

\section{Details of the patch-level breast cancer classifier}\label{details_classifyer}
In Section 3.2.1 of the main submission, we use a patch-level classifier to automatically generate low resolution labels. We show details of the classifier here.

The patch-level breast cancer classifier labels patches with probabilities of containing cancer. These probabilities are quantized to 10 bins as low resolution labels for label super resolution, since the probability of containing cancer given by a classifier is correlated with the percentage of cancer regions. We trained the classifier using 102 Whole Slide Images (WSIs) from the Surveillance, Epidemiology, and End Results (SEER) dataset as training data. A pathologist drew the boundaries of cancer regions in WSIs, generating a cancer region mask. To train the patch-level classifier, we extracted patches of $2000\times 2000$ pixels in 40X magnification. The label for each patch (0 or 1) was set by thresholding the ratio of cancer region in the patch by 0.5. We used ResNet34 \cite{He-et-al-CVPR16}, as the patch classification network. The resulting classifier was validated on a set of 7 WSIs and tested on a set of 89 WSIs. The DICE score between the prediction of this classifier and ground truth mask in the test set in \cite{HASHI} is 0.791.

For label super resolution in Section 3.2.1 of the main submission, we merge four $2000\times 2000$ patches into one $4000 \times 4000$ pixel image block. The low resolution label, quantized cancer probability, of an image block is the maximum probability among its 4 patches. The image block is then resized to $240 \times 240$ pixels for training the label super resolution network.

\section{Visual examples of breast cancer segmentation results}

Figure \ref{fig:breast1} show more breast cancer segmentation results.  The green lines are the segmentation boundaries by thresholding the low resolution probability scores for patches. The red lines are ground truth cancer boundaries given by pathologists. The blue lines are the cancer segmentation boundaries predicted by the proposed Intra+inter-instance LSR. The cyan lines are the the cancer segmentation boundaries predicted by the Intra-instance LSR baseline.

From those figures, we can see that the proposed Intra+inter-instance LSR predicts more continuous boundaries than the Intra-instance LSR baseline. Because given the low resolution label $z$ of a block, the Intra-instance LSR tries to match the count of pixels of cancer regions in each block with  $p(l|z)$ while the proposed Intra+inter-instance method considers the variance among blocks with the same low resolution label $z$. 

The segmentation results with super resolution are much closer to the ground truth than the low resolution results (green lines). It is to be noted that the annotation effort to train a super resolution model to super resolve from low resolution labels is much less than the effort for training a pixel-level supervised semantic segmentation model.

\begin{figure}
\centering
\begin{tabular}{c c}
\begin{subfigure}[b]{0.38\textwidth}
\includegraphics[width=\textwidth]{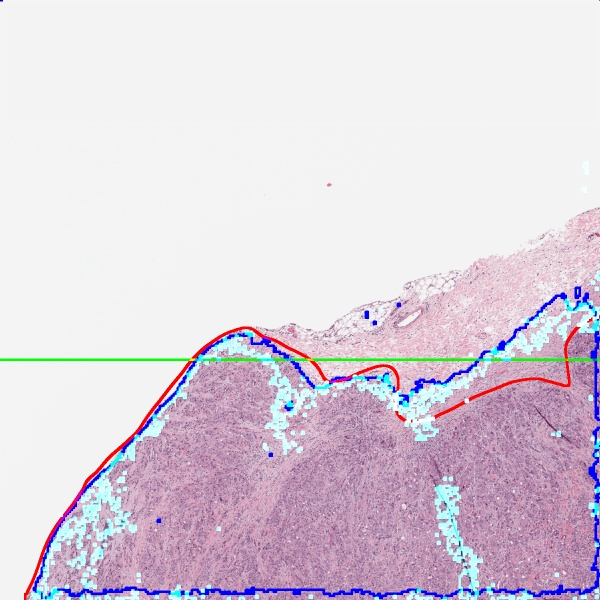}
%\caption{Picture 1}
%\label{fig:1}
\end{subfigure}&
\begin{subfigure}[b]{0.38\textwidth}
\includegraphics[width=\textwidth]{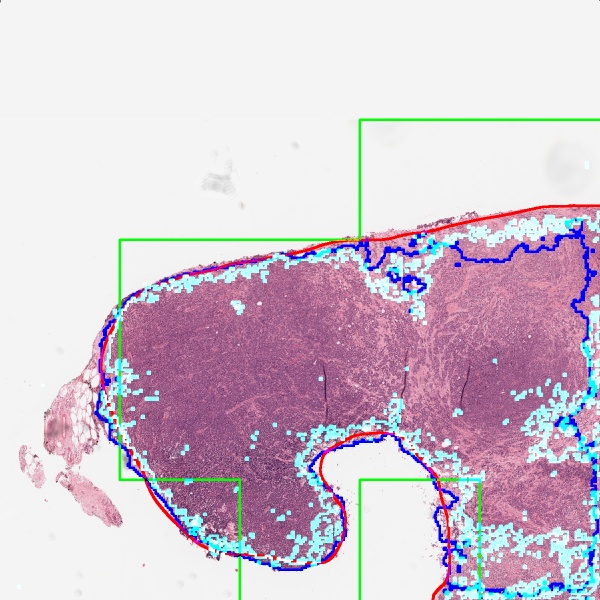}
%\caption{Picture 2}
%\label{fig:2}
\end{subfigure}\\
\begin{subfigure}[b]{0.38\textwidth}
\includegraphics[width=\textwidth]{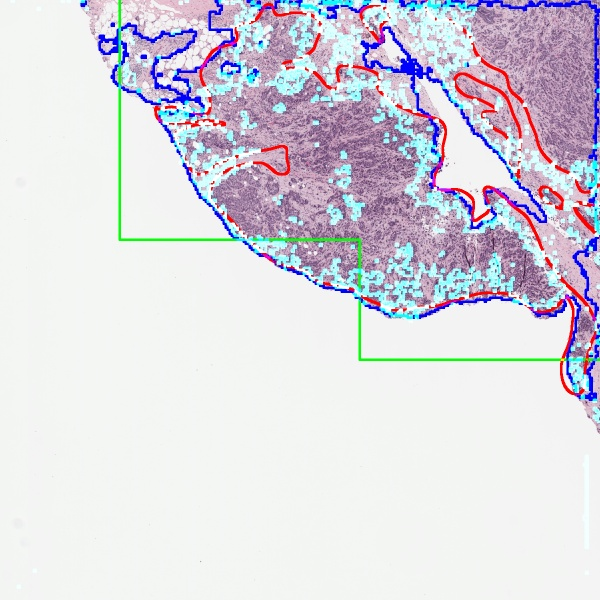}
%\caption{Picture 1}
%\label{fig:1}
\end{subfigure}&
\begin{subfigure}[b]{0.38\textwidth}
\includegraphics[width=\textwidth]{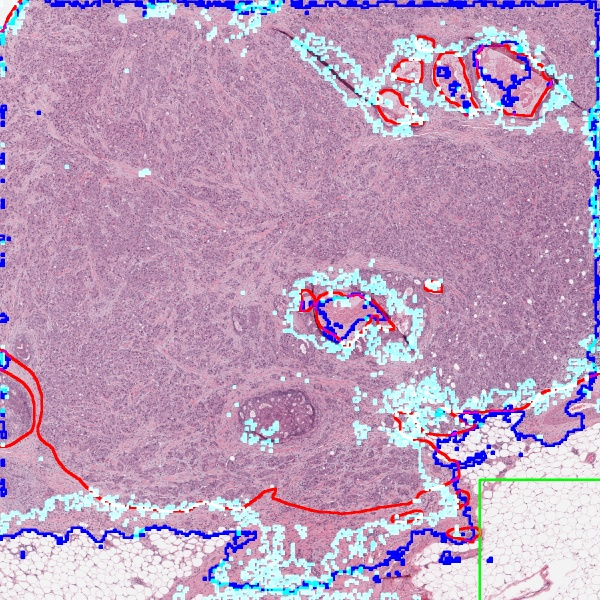}
%\caption{Picture 2}
%\label{fig:2}
\end{subfigure}\\
\begin{subfigure}[b]{0.38\textwidth}
\includegraphics[width=\textwidth]{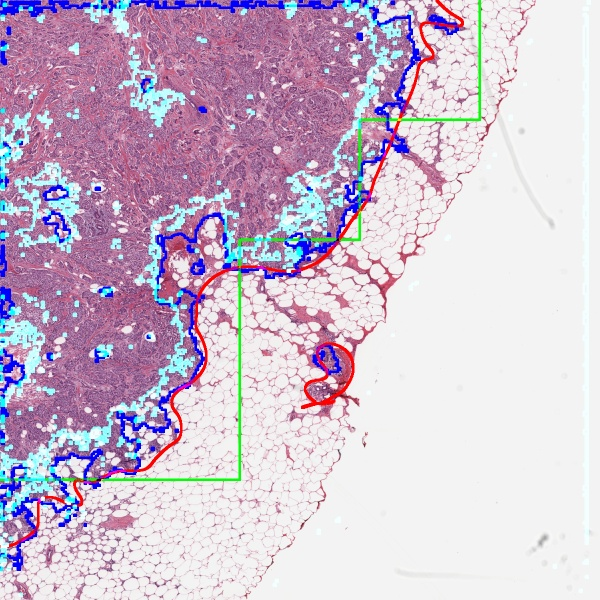}
%\caption{Picture 1}
%\label{fig:1}
\end{subfigure}&
\begin{subfigure}[b]{0.38\textwidth}
\includegraphics[width=\textwidth]{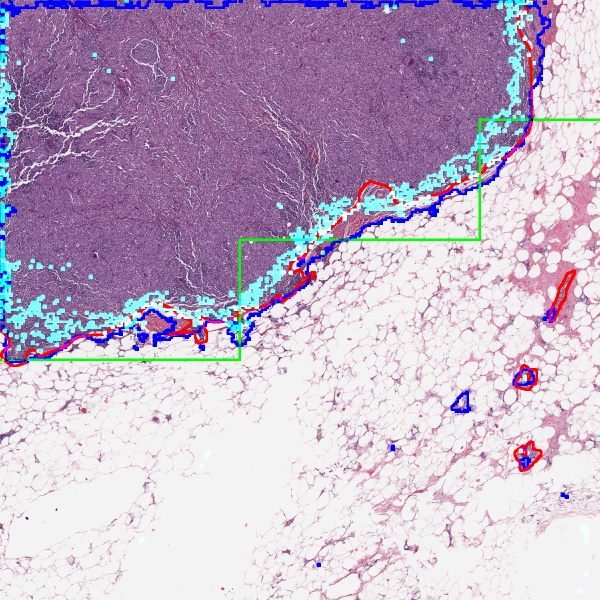}
%\caption{Picture 2}
%\label{fig:2}
\end{subfigure}\\
\end{tabular}
\caption{\label{fig:breast1}Visual examples of breast cancer segmentation. The green lines are the segmentation boundaries by thresholding the low resolution probability scores for patches . The red lines are ground truth cancer boundaries given by pathologists. The blue lines are the cancer segmentation boundaries predicted by the proposed Intra+inter-instance LSR. The cyan lines are the the cancer segmentation boundaries predicted by the Intra-instance LSR baseline.
   }
\end{figure}
